# Supplementary material for: As Biased as You Measure: Methodological Pitfalls of Bias Evaluations in Speaker Verification Research
Source: arXiv:2408.13614 source file (2024-08-24)
Supplement: Supplementary file 1 [file appendix.tex]

\section{Appendix}
